# Supplementary material for: Accuracy of the quantum regression theorem for photon emission from a quantum dot
Source: arXiv:2103.13100 ancillary file (2021-12-17)
Supplement: Supplementary file 1 [file Paper_QRT_erratum.pdf]

# Erratum: Accuracy of the quantum regression theorem for photon emission from a quantum dot

M. Cosacchi, T. Seidelmann, M. Cygorek, A. Vagov, D. E. Reiter, and V. M. Axt

In our Letter, the main investigation was a comparison between a numerically exact path-integral (PI) method and the quantum regression theorem (QRT) to model photonic figures of merit in quantum-dot–cavity systems obtained from two-time correlation functions. As a side aspect, we discussed the dependence of applying the quantum regression theorem in different frames, in particular, the lab frame and the polaron frame. The latter was achieved by considering the polaron master equation (PME) approach. Upon closer inspection of our numerical analysis, we have found a parameter error as explained below that affects the results obtained within the PME approach. We stress that the results do not affect the majority and the main message of the Letter, namely that the QRT overestimates the phonon influence on the indistinguishability. Nonetheless, the corrected results give rise to a number of additional insights regarding the PME approach that we would like to present in the following.

Concerning Fig. 2(c) of our original Letter, the numerically exact results and the ones obtained by using the QRT in the lab frame were calculated for a quantum dot (QD) with an electron confinement radius of $a_e = 3\,\mathrm{nm}$ (as defined in Tab. 1 in the supplemental material). In contrast, the PME results were erroneously calculated for $a_e = 4.175\,\mathrm{nm}$, which prohibits a meaningful comparison of the different methods. In Fig. 1, the corresponding PME results for a 3 nm QD are shown (blue dotted line).

As was stated in the original Letter, both the QRT applied in the lab frame and in the polaron frame systematically overestimate the phonon influence on the indistinguishability. In contrast to the previous comparison, though, quite unexpectedly the correct PME results basically coincide with the QRT results (cf., Fig. 1). Therefore, applying the QRT in the polaron frame does not improve the accuracy of the indistinguishability. This new insight calls for a more detailed explanation, which we would like to provide in the following in two subsequent steps: the comparison of numerically exact and PME results concerning single-time observables and then a discussion of the two-time correlation function $G^{(1)}(t,\tau) := \langle \sigma_X^+(t+\tau)\sigma_X \rangle$, which enters the definitions of both the QD emission spectrum and the indistinguishability $\mathcal{I}$.

In Fig. 2 the dynamics of the exciton occupation after resonant $\pi$-pulse excitation is shown. The numerically exact results are compared with the PME approach for two different phonon scalings $\lambda = 1$ and $\lambda = 10$. In the PME community, two different ways to account for the radiative decay by a phenomenological Lindblad term are being used: either the corresponding rate is scaled by a factor $\langle B\rangle^2$ (as done in, e.g., Ref. [85] of our Letter) or not (as done in, e.g., Ref. [87] of our Letter), where $\langle B\rangle$ is the phonon Franck-Condon factor as given in Eq. (15) in the supplemental material of our Letter. In the calculations shown in our Letter, we had scaled the radiative decay rate by the factor $\langle B\rangle^2$.

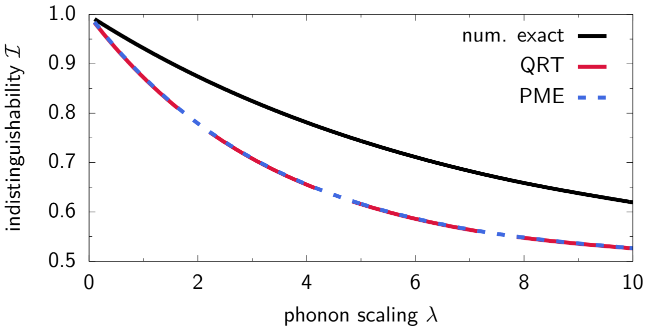


FIG. 1. The indistinguishability as a function of the phonon scaling parameter $\lambda$ at 4 K, calculated with the numerically exact path-integral method (num. exact), by using the QRT in the lab frame (QRT), and by applying the QRT in the polaron transformed frame within the PME approach (PME).

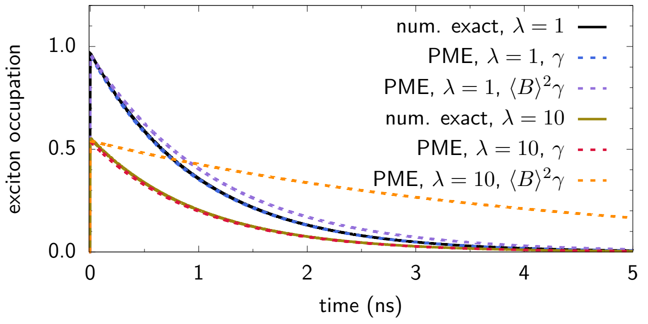


FIG. 2. The QD exciton dynamics at $T = 4\,\mathrm{K}$ after a Gaussian $\pi$-pulse of length $\tau_{\mathrm{fwhm}} = 3\,\mathrm{ps}$ centered around $t_0 = 0$. Numerically exact results are compared with PME results that either use a radiative decay rate of $\gamma$ or $\langle B\rangle^2\gamma$. The cases of two different phonon scalings $\lambda$ are shown.

Now, we show results for the exciton occupation obtained by both versions in Fig. 2. It becomes clear that the PME results without the additional factor $\langle B\rangle^2$ agree with the numerically exact path-integral results for both phonon scalings $\lambda$. Therefore, both methods take into account the phonon influence equally accurately concerning (single-time) expectation values. Since both the QRT

applied in the lab frame (labeled QRT in Fig. 1) and in the polaron frame (labeled PME in Fig. 1) introduce the same approximation to the method, this finding gives a first hint at the agreement between the two-time results obtained in the two frames.

Returning to Fig. 2, taking into account a rate $\langle B\rangle^2\gamma$ leads to results far off the path-integral calculations with an increasing difference for increasing phonon scaling $\lambda$. The underlying assumption that the radiative decay of the QD into a spectrally flat electromagnetic field environment is not affected by the phonon environment has recently been confirmed by taking into account both environements microscopically within the numerically exact algorithm ACE [M. Cygorek *et. al.*, arXiv:2101.01653 (2021)]. Therefore, we continue here without using the factor $\langle B\rangle^2$. (Note that the PME results in Fig. 1 are already calculated without $\langle B\rangle^2$. This different scaling, though, has only a marginal influence on the corresponding results for our parameters. The different QD size $a_e$ is responsible for the larger contribution to the change of the results.)

In Fig. 3, which corresponds to Fig. 1 in the supplemental material of our Letter, we show an emission spectrum obtained within the PME formalism without the factor $\langle B\rangle^2$ (blue dotted line). All other curves are the same as in the original figure. Strikingly, the PME spectrum is now almost a mirror image of the spectrum obtained by applying the QRT in the lab frame (red dashed line) similar to what was found earlier by a perturbative approach (cf., Ref. [26] of our Letter). Since the emission spectrum is essentially the Fourier transform of the two-time correlation function $G^{(1)}(t,\tau)$ [cf., Eq. (13) in the supplemental material of our Letter], this finding implies that using the QRT in the lab or in the polaron frame affects essentially only the sign of the imaginary part of $G^{(1)}(t,\tau)$. We stress that there is a sizable quantitative difference between the spectra resulting from the numerically exact and the PME approaches. This difference arises because the QRT applied in the polaron frame is overestimating the phonon influence on the correlation function $G^{(1)}(t,\tau)$.

With the conclusions drawn from Figs. 2 and 3, we can now explain, why the QRT applied in the lab and in the polaron frame agree concerning the indistinguishability $\mathcal{I}$ in Fig. 1. The indistinguishability is based upon the Hong-Ou-Mandel correlation function

$$G^{(2)}_{\mathrm{HOM}}(t,\tau) := \frac{1}{2}\left[\langle\sigma_X^\dagger(t)\sigma_X(t)\rangle\langle\sigma_X^\dagger(t+\tau)\sigma_X(t+\tau)\rangle - \left|\langle\sigma_X^\dagger(t+\tau)\sigma_X(t)\rangle\right|^2 + G^{(2)}(t,\tau)\right] \quad (1)$$

[cf., Eqs. (3) and (4) in our Letter]. We now look at each term of this expression and compare their derivation within the different methods. The factors in the first term are both (single-time) expectation values of the exciton occupation. Fig. 2 gives a compelling argument that the PME approach agrees well with the path-integral method regarding the exciton occupation for the parameters concerned. The last term is the second-order two-time correlation function $G^{(2)}(t,\tau)$, upon which the single-photon purity $\mathcal{P}$ is based. In our Letter, we found that the QRT introduces basically no error to this quantity compared with the numerically exact evaluation of the two-time function. The second term $|\langle\sigma_X^\dagger(t+\tau)\sigma_X(t)\rangle|^2$ is the absolute square of the first-order correlation function $G^{(1)}(t,\tau)$. Fig. 3 implies that the QRT and PME results differ basically only by the sign of the imaginary part of this correlation function, which does not affect the absolute square. Thus, we find that for all three terms there is no difference between the QRT and the PME. This is the reason why the QRT and PME results of the indistinguishability $\mathcal{I}$ are in such good agreement in Fig. 1. However, the large difference between the numerically exact results and the QRT approximation remains. It stems from the already noticed quantitative difference in the $G^{(1)}(t,\tau)$ function as observed earlier in the spectra. This implies that the only error resulting in a reduced indistinguishability is caused solely by the application of the QRT, regardless of the frame it is used in.

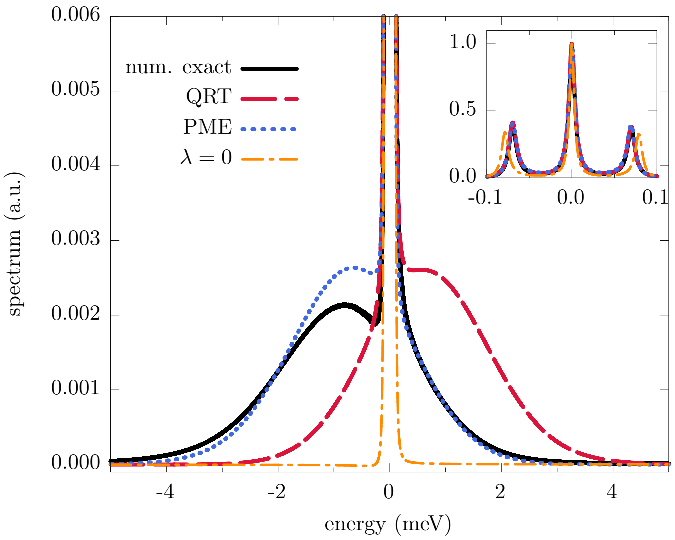


FIG. 3. The QD emission spectrum calculated for a constantly driven QD with $\hbar f_{\mathrm{p}}(t) = 0.079\,\mathrm{meV}$ and a radiative decay rate of $\gamma = 0.01\,\mathrm{ps}^{-1}$ at $T = 10\,\mathrm{K}$. The numerically exact result (num. exact) is compared with results obtained using the quantum regression theorem in the lab frame (QRT) and in the polaron frame (PME). In the latter, an unscaled radiative decay rate $\gamma$ is used instead of a factor $\langle B\rangle^2\gamma$ as in the original plot (Fig. 1 in the supplemental material of our Letter). As a reference, the phonon-free case $\lambda = 0$ is also shown. The inset depicts the same data on a different scale, where the Mollow triplet becomes visible.

Therefore, our correction sheds new light on the PME formalism: For the considered parameters, the PME re-

sults concerning (single-time) expectation values match the numerically exact path-integral calculations well. Nonetheless, a large difference is found regarding the indistinguishability, which is based upon two-time correlation functions, the highest relative error being 18 % in the parameter space under scrutiny. Finally, the impact of the application of the QRT on the indistinguishability is independent of the frame: Applying the QRT in the polaron frame does not yield an improvement of the prediction of the indistinguishability.
