# Supplementary material for: Accuracy of the quantum regression theorem for photon emission from a quantum dot
Source: arXiv:2103.13100 ancillary file (2021-12-17)
Supplement: Supplementary file 2 [file Paper_QRT_supplement.pdf]

# Supplement: Accuracy of the quantum regression theorem for photon emission from a quantum dot

M. Cosacchi,[1] T. Seidelmann,[1] M. Cygorek,[2] A. Vagov,[1,3] D. E. Reiter,[4] and V. M. Axt[1]
[1] *Theoretische Physik III, Universität Bayreuth, 95440 Bayreuth, Germany*
[2] *Heriot-Watt University, Edinburgh EH14 4AS, United Kingdom*
[3] *ITMO University, St. Petersburg, 197101, Russia*
[4] *Institut für Festkörpertheorie, Universität Münster, 48149 Münster, Germany*

## I. HAMILTONIAN AND MODEL EQUATION

Our model Hamiltonian reads as:

$$H = H_{\mathrm{QD}} + H_{\mathrm{Ph}} + H_{\mathrm{driving}}\,. \tag{1}$$

The two-level quantum dot (QD) has an excited state $|X\rangle$ at energy $\hbar\omega_X$ and the energy of the ground state $|G\rangle$ is set to zero. In a frame co-rotating with the laser frequency $\omega_L$ the corresponding Hamiltonian is

$$H_{\mathrm{QD}} = \hbar\Delta\omega_{XL}|X\rangle\langle X| \tag{2}$$

with the exciton-laser detuning $\Delta\omega_{XL} = \omega_X - \omega_L$. The QD interacts with an environment of longitudinal acoustic (LA) phonons via a pure-dephasing coupling Hamiltonian [1–5]

$$H_{\mathrm{Ph}} = \hbar\sum_{\mathbf{q}}\omega_{\mathbf{q}}b^\dagger_{\mathbf{q}}b_{\mathbf{q}} + \hbar\sqrt{\lambda}\sum_{\mathbf{q}}\left(\gamma^{\mathrm{X}}_{\mathbf{q}}b^\dagger_{\mathbf{q}} + \gamma^{\mathrm{X}*}_{\mathbf{q}}b_{\mathbf{q}}\right)|X\rangle\langle X|\,, \tag{3}$$

where $b_{\mathbf{q}}$ ($b^\dagger_{\mathbf{q}}$) annihilates (creates) a phonon in the mode $\mathbf{q}$ with energy $\hbar\omega_{\mathbf{q}}$. The coupling strength to the QD is denoted by $\gamma^{\mathrm{X}}_{\mathbf{q}}$. In order to analyze the impact of the phonon coupling, we introduce a scaling parameter $\lambda$, with $0 \le \lambda \le 10$. $\lambda = 0$ describes the phonon-free case, $\lambda = 1$ the coupling in a GaAs QD. $1 < \lambda \le 10$ roughly estimates the stronger phonon coupling in piezoelectric materials like GaN [6]. $\lambda$ is referred to as the phonon scaling in the main text. Note that we followed the standard way to write the phonon coupling in Eq. (3) to the exciton state $|X\rangle$ only. But in fact, it can be written to the ground state $|G\rangle$ without any influence on the stationary emission spectrum, which we checked numerically by calculating the QRT spectrum in Fig. 1 (red dashed line) both ways.

The QD is driven by an external laser pulse described by

$$H_{\mathrm{driving}} = -\frac{\hbar}{2}f_{\mathrm{p}}(t)\left(\sigma_X + \sigma_X^\dagger\right)\,. \tag{4}$$

$\sigma_X := |G\rangle\langle X|$ is the operator for the transition between $|X\rangle$ and the ground state $|G\rangle$. $f_{\mathrm{p}}(t)$ is the real envelope function of the external laser pulse. Throughout the main text, we consider a Gaussian pulse with an area of $\pi$ and pulse duration as measured by the full width at half maximum $\tau_{\mathrm{FWHM}} = 3\,\mathrm{ps}$ resonant to the polaron shifted QD transition energy. We further account for the radiative decay of the QD exciton by introducing a Lindblad superoperator acting on the density matrix $\rho$ to our model

$$\mathcal{L}_{\sigma_X,\gamma}\rho = \gamma\left(\sigma_X\rho\sigma_X^\dagger - \frac{1}{2}\left\{\rho,\sigma_X^\dagger\sigma_X\right\}_+\right)\,, \tag{5}$$

where $\{A,B\}_+$ denotes the anti-commutator of operators $A$ and $B$ and $\gamma$ the radiative decay rate set to a typical value of $1\,\mathrm{ns}^{-1}$ unless noted otherwise.

In this model the QD environment consists of two parts: the coupling to photon modes which is responsible for the radiative decay and the coupling to phonons. Since the radiative decay is modeled by a Markovian rate, it is not expected to limit the validity of the QRT. Phonons are known to influence the QD dynamics profoundly [1, 7–18] and to be the origin of non-Markovian behavior [5, 19–23], which might entail errors of the QRT.

While the Hamiltonian in Eq. (1) defines the model, the corresponding Liouville-von Neumann equation for the density matrix $\rho$ reads

$$\frac{\partial}{\partial t}\rho = -\frac{i}{\hbar}\{H,\rho\}_- + \mathcal{L}_{\sigma_X,\gamma}\rho \tag{6}$$

TABLE I. Parameters typical for GaAs QDs [6].

| | | |
|---|---|---|
| Electron deformation potential | $D_e$ (eV) | 7.0 |
| Hole deformation potential | $D_h$ (eV) | -3.5 |
| Density | $\rho_D$ (kg/m$^3$) | 5370 |
| Sound velocity | $c_s$ (m/s) | 5110 |
| Electron-to-hole confinement ratio | $a_e/a_h$ | 1.15 |
| Electron confinement radius | $a_e$ (nm) | 3.0 |

with the commutator $\{A, B\}_-$ of operators $A$ and $B$. This equation is solved in a numerically exact way for the time evolution of the QD subsystem's reduced density matrix $\bar{\rho} = \mathrm{Tr}_{\mathrm{Ph}}[\rho]$, where the trace is taken over the phonon subspace, by employing an iterative real-time path-integral formalism (details are explained in Refs. 24–26).

The deformation potential coupling of the QD to LA phonons influences the reduced electronic density matrix via the phonon spectral density $J(\omega) = \sum_{\mathbf{q}} |\gamma_{\mathbf{q}}^X|^2 \delta(\omega - \omega_{\mathbf{q}})$. Note that the sign or even the phase of the coupling has no influence on the electronic dynamics, since only the absolute square enters the spectral density. Assuming a linear dispersion $\omega_{\mathbf{q}} = c_s|\mathbf{q}|$ with sound velocity $c_s$ and Gaussian wave functions for both electrons and holes with radii $a_e$ and $a_h$, the spectral density becomes [24, 26, 27]

$$J(\omega) = \frac{\omega^3}{4\pi^2 \rho_D \hbar c_s^5} \left( D_e e^{-\omega^2 a_e^2/(4c_s^2)} - D_h e^{-\omega^2 a_h^2/(4c_s^2)} \right)^2 . \tag{7}$$

We use typical GaAs parameters for a QD with radius $a_e = 3.0\,\mathrm{nm}$ listed in Tab. I. Note that scaling the phonon coupling $\gamma_{\mathbf{q}}^X$ with $\sqrt{\lambda}$ as in Eq. (3) implies that the spectral density $J(\omega)$ is scaled with $\lambda$.

The low-frequency behavior of this spectral density is given by $J(\omega) \propto \omega^s$ with $s = 3$. Spectral densities with such a power law dependence are classified as super-Ohmic, in contrast to the Ohmic case, for which $s = 1$, and the sub-Ohmic case with $0 \leq s < 1$. The super-Ohmic case is known to result in a nonexponential and only partial polarization decay [3] which is a clear signature of non-Markovian dynamics. Rather generally, the low-frequency behavior has been shown to potentially play a decisive role for the relation between Markovianity and QRT errors [28].

## II. EVALUATION OF $G^{(2)}(t, \tau)$

**Numerically Exact Evaluation** To evaluate the two-time correlation function introduced in the main text $G^{(2)}(t,\tau) = \langle \sigma_X^\dagger(t)\sigma_X^\dagger(t+\tau)\sigma_X(t+\tau)\sigma_X(t)\rangle$ within the path-integral formalism, first, we assume a time discretization of $n$ equidistant time steps with length $\Delta t$ for the interval $[0,t]$ and of another $m$ time steps of the same length to cover $[t, t+\tau]$, i.e., $t = n\Delta t$ and $\tau = m\Delta t$. The object propagated in time is the augmented density matrix (ADM), a $2n_c$-rank tensor that contains all the information induced by the $n_c\Delta t$ long memory. The iterative propagation of the ADM is summarized as [25]:

$$\bar{\rho}_{\nu_n \dots \nu_{n-n_c+1}}^{\mu_n \dots \mu_{n-n_c+1}} = \mathcal{M}_{\nu_n \mu_n}^{\nu_{n-1}\mu_{n-1}} \sum_{\substack{\nu_{n-n_c} \\ \mu_{n-n_c}}} \exp\left( \sum_{l=n-n_c}^{n} S_{\nu_n \nu_l \mu_n \mu_l} \right) \bar{\rho}_{\nu_{n-1}\dots\nu_{n-n_c}}^{\mu_{n-1}\dots\mu_{n-n_c}} , \tag{8}$$

where $\mathcal{M}_{\nu_n \mu_n}^{\nu_{n-1}\mu_{n-1}}$ is the subsystem propagator and $S_{\nu_n \nu_l \mu_n \mu_l}$ the phonon influence functional. The indices $\mu_j$ and $\nu_j$ describe the subsystem state $\mu$ and $\nu$, respectively, at the time step $j$. The subsystem's reduced density matrix at time $n\Delta t$, which is the quantity necessary to calculate any expectation value of observables within the subsystem, is obtained by tracing out the memory contained in the ADM, i.e.,

$$\bar{\rho}_{\nu_n \mu_n} = \sum_{\substack{\nu_{n-1}\dots\nu_{n-n_c+1} \\ \mu_{n-1}\dots\mu_{n-n_c+1}}} \bar{\rho}_{\nu_n \dots \nu_{n-n_c+1}}^{\mu_n \dots \mu_{n-n_c+1}} . \tag{9}$$

In order to calculate the two-time correlation function $G^{(2)}(t,\tau)$, the ADM is propagated for the first $n$ steps, after

which the operators evaluated at time $t$ are multiplied to produce a modified ADM (MADM):

$$\bar{\rho}_{\sigma_X\sigma_X^\dagger \nu_n\cdots\nu_{n-n_c+1}}^{\quad\mu_n\cdots\mu_{n-n_c+1}} = \sum_{\nu_n'\mu_n'} (\sigma_X)_{\nu_n\nu_n'} \mathcal{M}_{\nu_n'\mu_n'}^{\nu_{n-1}\mu_{n-1}} (\sigma_X^\dagger)_{\mu_n'\mu_n} \sum_{\substack{\nu_{n-n_c}\\ \mu_{n-n_c}}} \exp\left(\sum_{l=n-n_c}^{n} S_{\nu_n\nu_l\mu_n\mu_l}\right) \bar{\rho}_{\nu_{n-1}\cdots\nu_{n-n_c}}^{\mu_{n-1}\cdots\mu_{n-n_c}}\,, \tag{10}$$

The MADM follows the same recursion as the ADM, such that for the subsequent $m$ steps until $t+\tau$, the MADM is iterated instead of the ADM. Finally, the two-time correlation function is obtained by multiplying the operators evaluated at time $t+\tau$ and the trace is performed to yield

$$G^{(2)}(t,\tau) = \sum_{\substack{\nu_{n+m}\cdots\nu_{n+m-n_c+1}\\ \mu_{n+m}\cdots\mu_{n+m-n_c+1}}} \left[\sigma_X^\dagger\sigma_X\right]_{\mu_{n+m}\nu_{n+m}} \bar{\rho}_{\sigma_X\sigma_X^\dagger \nu_{n+m}\cdots\nu_{n+m-n_c+1}}^{\quad\mu_{n+m}\cdots\mu_{n+m-n_c+1}}\,. \tag{11}$$

A derivation of this scheme with detailed explanations can be found in Ref. [29]. Note that the first-order correlation function $\langle\sigma_X^\dagger(t+\tau)\sigma_X(t)\rangle$ appearing in the main text can be obtained using the same method by simply exchanging $\sigma_X^\dagger(t)$ and $\sigma_X(t+\tau)$ with identity operators in $G^{(2)}(t,\tau)$.

**QRT Evaluation** To implement the QRT within this framework, one traces out the memory of the ADM after reaching the time $n\Delta t$ as in Eq. (9) to obtain the reduced density matrix (RDM) $\bar{\rho}_{\nu_n\mu_n}$. Then, a modified RDM (MRDM) which is defined as

$$\bar{\rho}_{\sigma_X\sigma_X^\dagger\nu_n}^{\quad\mu_n} = \sum_{\nu_n'\mu_n'} (\sigma_X)_{\nu_n\nu_n'} \bar{\rho}_{\nu_n'\mu_n'} (\sigma_X^\dagger)_{\mu_n'\mu_n} \tag{12}$$

is used as the new initial RDM for the next $m$ time steps, which now describe the propagation in $\tau$. The essential difference to the exact propagation scheme is that here the memory acquired until the time $t$ is discarded for the subsequent $\tau$-propagation. As for the initial (real) time $t=0$, the phonon subspace is assumed to be in equilibrium at a temperature of $T$ at the time $n\Delta t$, when the propagation of the MRDM begins. The statistical operator of the total system is approximated by the QRT at the beginning of the $\tau$-propagation by a product of the statistical operators for the two-level system and the environment, thus ignoring the entanglement between these subsystems that has been built up during the $t$-propagation due to their mutual interaction [30].

## III. EMISSION SPECTRA AND QRT IMPLEMENTATION

The emission spectrum $S(\omega)$ is obtained in a stationary nonequilibrium state of the system. To this end, the first-order two-time correlation function $G^{(1)}(t,\tau) = \langle\sigma_X^\dagger(t+\tau)\sigma_X(t)\rangle$ is considered in the limit $t\to\infty$. After subtraction of the coherent part of the emission [29, 31] $\lim_{t,\tau\to\infty} G^{(1)}(t,\tau)$ the Fourier transform is taken:

$$S(\omega) = \mathrm{Re}\left[\int_{-\infty}^{\infty} d\tau \lim_{t\to\infty}\left(G^{(1)}(t,\tau) - \lim_{\tau\to\infty} G^{(1)}(t,\tau)\right) e^{-i\omega\tau}\right]\,. \tag{13}$$

In Fig. 1 QD emission spectra calculated for a constantly driven QD with a field strength of $\hbar f_\mathrm{p}(t) = 0.079\,\mathrm{meV}$ and a radiative decay rate of $\gamma = 0.01\,\mathrm{ps}^{-1}$ at $T = 10\,\mathrm{K}$ are shown. As a reference, the phonon-free result, i.e., for $\lambda = 0$, is depicted (orange dashed-dotted line), where no sidebands appear. The inset in Fig. 1 shows the same data zoomed in on the energy scale and zoomed out on the intensity axis. On this scale, the Mollow triplet becomes visible with the peaks at $\pm\hbar f_\mathrm{p}$, which corresponds to the Rabi splitting. For finite temperature, the peaks shift to smaller energies and broaden slightly, which corresponds to the phonon-induced renormalization of the Rabi frequency and its damping, respectively. Note that the numerically exact result at 10 K has been obtained by employing a matrix-product-state representation of the iterative path-integral method [32] to enable calculations with very fine time discretization.

We stress that there is a clear physical picture that the phonon sideband has to be on the left side of the zero phonon line (ZPL). At low temperatures, phonon emission is strongly favored over phonon absorption. Therefore, the energies of the emitted photon and of the emitted phonon have to add up to the QD transition energy due to energy conservation. Accordingly, in an emission spectrum, the energy of the emitted photon after phonon emission has to be smaller than the QD transition energy. This results in the phonon emission sideband being on the energetically lower side of the ZPL.

The numerically exact approach (black solid line) gives the physically correct results showing the phonon sideband on the energetically lower side of the ZPL. In contrast, when the QRT is applied, the phonon sideband appears on

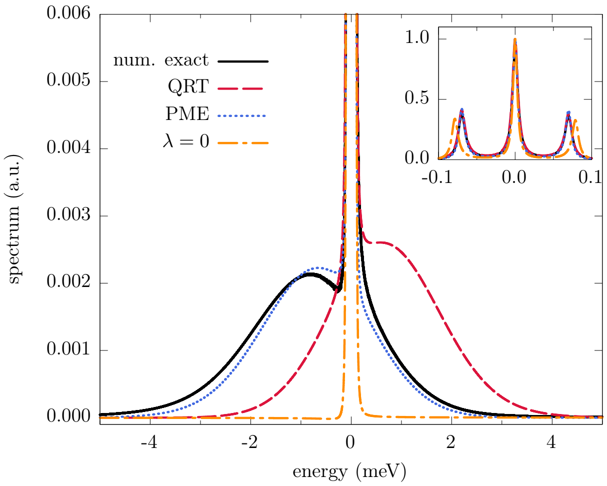


FIG. 1. The QD emission spectrum [29] calculated for a constantly driven QD with $\hbar f_\mathrm{p}(t) = 0.079\,\mathrm{meV}$ and a radiative decay rate of $\gamma = 0.01\,\mathrm{ps}^{-1}$ at $T = 10\,\mathrm{K}$. The numerically exact result (num. exact) is compared with results obtained using the QRT in the lab frame (QRT) and in the polaron frame (PME). As a reference, the phonon-free case $\lambda = 0$ is also shown. The inset depicts the same data on a different scale, where the Mollow triplet becomes visible.

the energetically higher side (red dashed line). This wrong outcome of the QRT was already discussed in Ref. 22, where it was explicitly shown that by neglecting correlations resulting in memory effects, physically wrong results are obtained. We consider our implementation of the QRT as verified, since it reproduces this result of Ref. 22, which was obtained within a completely different methodological framework. When including said correlations and memory effects on the other hand, as they are in our numerically exact path-integral approach, the physically correct picture of a phonon sideband at the lower energy side of the emission spectrum is found.

## IV. THE QRT IN THE POLARON TRANSFORMED FRAME

An approximate method to account for the coupling to the LA phonon environment is the polaron master equation approach (PME) [33–35]. The core idea of this method is to transform the system into the polaron frame by

$$H' = e^S H e^{-S} \tag{14a}$$

$$S = \sigma_X^\dagger \sigma_X \sum_\mathbf{q} \frac{\sqrt{\lambda}}{\omega_\mathbf{q}} \left(\gamma_\mathbf{q}^X b_\mathbf{q}^\dagger - \gamma_\mathbf{q}^{X*} b_\mathbf{q}\right) . \tag{14b}$$

Only then the Markov approximation is employed to obtain a time-local master equation for the reduced subsystem dynamics. This method becomes exact in the weak-driving limit. Since we consider strong pulsed excitation, it is not a priori clear if this condition is fulfilled. The PME approach captures a variety of non-Markovian features that would be lost if the Markov approximation had been used in the original laboratory frame.

Therefore, the question arises whether the QRT is also frame dependent. Indeed, QD emission spectra calculated within the PME approach by employing the QRT in the polaron frame show the correct phonon sidebands [36], cf., blue dotted line in Fig. 1.

In the following, we describe the procedure to compare the effect of using the QRT in the lab and the polaron frame on the indistinguishability, cf., Fig. 2(c) in the main text. To obtain the indistinguishability in the lab frame within the PME approach, one has to transform it back after using the QRT in the polaron frame. In this transformation, all $\sigma_X^\dagger$ ($\sigma_X$) operators acquire a $B_+$ ($B_-$) operator with $B_\pm = \exp\left[\pm\sum_\mathbf{q}(\sqrt{\lambda}/\omega_\mathbf{q})(\gamma_\mathbf{q}^{X*} b_\mathbf{q} - \gamma_\mathbf{q}^X b_\mathbf{q}^\dagger)\right]$. Hence, whenever the two transition operators appear in pairs at equal times as in the second-order correlation function $G^{(2)}(t,\tau)$ the back transform is the identity operation. In contrast, the function $G^{(1)}(t,\tau)$ is influenced by the back transform. In particular, a term $\langle B_+(\tau)B_-(0)\rangle$ appears, which is simplified to $\langle B\rangle^2 e^{\phi(\tau)}$ [37]. The so-called Franck-Condon factor

[16] $\langle B\rangle$ is defined as

$$\langle B\rangle = \langle B_{\pm}\rangle = \exp\left[-\frac{1}{2}\int_0^{\infty} d\omega \frac{J(\omega)}{\omega^2}\coth\left(\hbar\omega/(2k_BT)\right)\right], \tag{15}$$

where $k_B$ denotes the Boltzmann constant. The phonon correlation function is

$$\phi(\tau) = \int_0^{\infty} d\omega \frac{J(\omega)}{\omega^2}\left[\coth\left(\hbar\omega/(2k_BT)\right)\cos\left(\omega\tau\right) - i\sin\left(\omega\tau\right)\right]. \tag{16}$$

---


[1] L. Besombes, K. Kheng, L. Marsal, H. Mariette. 'Acoustic phonon broadening mechanism in single quantum dot emission'. *Phys. Rev. B* **63**, 155307 (2001). doi:10.1103/PhysRevB.63.155307.

[2] P. Borri, W. Langbein, S. Schneider, U. Woggon, R. L. Sellin, D. Ouyang, D. Bimberg. 'Ultralong dephasing time in InGaAs quantum dots'. *Phys. Rev. Lett.* **87**, 157401 (2001). doi:10.1103/PhysRevLett.87.157401.

[3] B. Krummheuer, V. M. Axt, T. Kuhn. 'Theory of pure dephasing and the resulting absorption line shape in semiconductor quantum dots'. *Phys. Rev. B* **65**, 195313 (2002). doi:10.1103/PhysRevB.65.195313.

[4] V. M. Axt, T. Kuhn, A. Vagov, F. M. Peeters. 'Phonon-induced pure dephasing in exciton-biexciton quantum dot systems driven by ultrafast laser pulse sequences'. *Phys. Rev. B* **72**, 125309 (2005). doi:10.1103/PhysRevB.72.125309.

[5] D. E. Reiter, T. Kuhn, V. M. Axt. 'Distinctive characteristics of carrier-phonon interactions in optically driven semiconductor quantum dots'. *Adv. Phys.: X* **4**, 1655478 (2019). doi:10.1080/23746149.2019.1655478.

[6] B. Krummheuer, V. M. Axt, T. Kuhn, I. D'Amico, F. Rossi. 'Pure dephasing and phonon dynamics in GaAs- and GaN-based quantum dot structures: Interplay between material parameters and geometry'. *Phys. Rev. B* **71**, 235329 (2005). doi:10.1103/PhysRevB.71.235329.

[7] J. Förstner, C. Weber, J. Danckwerts, A. Knorr. 'Phonon-assisted damping of rabi oscillations in semiconductor quantum dots'. *Phys. Rev. Lett.* **91**, 127401 (2003). doi:10.1103/PhysRevLett.91.127401.

[8] P. Machnikowski, L. Jacak. 'Resonant nature of phonon-induced damping of Rabi oscillations in quantum dots'. *Phys. Rev. B* **69**, 193302 (2004). doi:10.1103/PhysRevB.69.193302.

[9] A. Vagov, V. M. Axt, T. Kuhn, W. Langbein, P. Borri, U. Woggon. 'Nonmonotonous temperature dependence of the initial decoherence in quantum dots'. *Phys. Rev. B* **70**, 201305(R) (2004). doi:10.1103/PhysRevB.70.201305.

[10] A. Vagov, M. D. Croitoru, V. M. Axt, T. Kuhn, F. M. Peeters. 'Nonmonotonic field dependence of damping and reappearance of Rabi oscillations in quantum dots'. *Phys. Rev. Lett.* **98**, 227403 (2007). doi:10.1103/PhysRevLett.98.227403.

[11] A. J. Ramsay, A. V. Gopal, E. M. Gauger, A. Nazir, B. W. Lovett, A. M. Fox, M. S. Skolnick. 'Damping of exciton Rabi rotations by acoustic phonons in optically excited InGaAs/GaAs quantum dots'. *Phys. Rev. Lett.* **104**, 017402 (2010). doi:10.1103/PhysRevLett.104.017402.

[12] M. Florian, P. Gartner, C. Gies, F. Jahnke. 'Phonon-mediated off-resonant coupling effects in semiconductor quantum-dot lasers'. *New J. Phys.* **15**, 035019 (2013). doi:10.1088/1367-2630/15/3/035019.

[13] A. Nysteen, P. Kaer, J. Mork. 'Proposed quenching of phonon-induced processes in photoexcited quantum dots due to electron-hole asymmetries'. *Phys. Rev. Lett.* **110**, 087401 (2013). doi:10.1103/PhysRevLett.110.087401.

[14] D. P. S. McCutcheon, A. Nazir. 'Model of the optical emission of a driven semiconductor quantum dot: Phonon-enhanced coherent scattering and off-resonant sideband narrowing'. *Phys. Rev. Lett.* **110**, 217401 (2013). doi: 10.1103/PhysRevLett.110.217401.

[15] D. E. Reiter, T. Kuhn, M. Glässl, V. M. Axt. 'The role of phonons for exciton and biexciton generation in an optically driven quantum dot'. *Journal of Physics: Condensed Matter* **26**, 423203 (2014). doi:10.1088/0953-8984/26/42/423203.

[16] J. Iles-Smith, D. P. S. McCutcheon, A. Nazir, J. Mørk. 'Phonon scattering inhibits simultaneous near-unity efficiency and indistinguishability in semiconductor single-photon sources'. *Nature Photonics* **11**, 521 (2017). doi:10.1038/nphoton.2017.101.

[17] T. Kaldewey, S. Lüker, A. V. Kuhlmann, S. R. Valentin, J.-M. Chauveau, A. Ludwig, A. D. Wieck, D. E. Reiter, T. Kuhn, R. J. Warburton. 'Demonstrating the decoupling regime of the electron-phonon interaction in a quantum dot using chirped optical excitation'. *Phys. Rev. B* **95**, 241306 (2017). doi:10.1103/PhysRevB.95.241306.

[18] M. Reindl, K. D. Jöns, D. Huber, C. Schimpf, Y. Huo, V. Zwiller, A. Rastelli, R. Trotta. 'Phonon-assisted two-photon interference from remote quantum emitters'. *Nano Lett.* **17**, 4090 (2017). doi:10.1021/acs.nanolett.7b00777.

[19] P. Kaer, T. R. Nielsen, P. Lodahl, A.-P. Jauho, J. Mørk. 'Non-Markovian Model of Photon-Assisted Dephasing by Electron-Phonon Interactions in a Coupled Quantum-Dot-Cavity System'. *Phys. Rev. Lett.* **104**, 157401 (2010). doi: 10.1103/PhysRevLett.104.157401.

[20] D. P. S. McCutcheon, A. Nazir. 'Quantum dot Rabi rotations beyond the weak exciton–phonon coupling regime'. *New Journal of Physics* **12**, 113042 (2010). doi:10.1088/1367-2630/12/11/113042.

[21] P. Kaer, P. Lodahl, A.-P. Jauho, J. Mork. 'Microscopic theory of indistinguishable single-photon emission from a quantum dot coupled to a cavity: The role of non-Markovian phonon-induced decoherence'. *Phys. Rev. B* **87**, 081308 (2013). doi:10.1103/PhysRevB.87.081308.

[22] D. P. S. McCutcheon. 'Optical signatures of non-Markovian behavior in open quantum systems'. *Phys. Rev. A* **93**, 022119 (2016). doi:10.1103/PhysRevA.93.022119.

[23] A. Carmele, S. Reitzenstein. 'Non-Markovian features in semiconductor quantum optics: quantifying the role of phonons in experiment and theory'. *Nanophotonics* **8**, 655 (2019). doi:doi:10.1515/nanoph-2018-0222.
[24] A. Vagov, M. D. Croitoru, M. Glässl, V. M. Axt, T. Kuhn. 'Real-time path integrals for quantum dots: Quantum dissipative dynamics with superohmic environment coupling'. *Phys. Rev. B* **83**, 094303 (2011). doi:10.1103/PhysRevB.83.094303.
[25] A. M. Barth, A. Vagov, V. M. Axt. 'Path-integral description of combined Hamiltonian and non-Hamiltonian dynamics in quantum dissipative systems'. *Phys. Rev. B* **94**, 125439 (2016). doi:10.1103/PhysRevB.94.125439.
[26] M. Cygorek, A. M. Barth, F. Ungar, A. Vagov, V. M. Axt. 'Nonlinear cavity feeding and unconventional photon statistics in solid-state cavity QED revealed by many-level real-time path-integral calculations'. *Phys. Rev. B* **96**, 201201(R) (2017). doi:10.1103/PhysRevB.96.201201.
[27] S. Lüker, T. Kuhn, D. E. Reiter. 'Phonon impact on optical control schemes of quantum dots: Role of quantum dot geometry and symmetry'. *Phys. Rev. B* **96**, 245306 (2017). doi:10.1103/PhysRevB.96.245306.
[28] G. Guarnieri, A. Smirne, B. Vacchini. 'Quantum regression theorem and non-Markovianity of quantum dynamics'. *Phys. Rev. A* **90**, 022110 (2014). doi:10.1103/PhysRevA.90.022110.
[29] M. Cosacchi, M. Cygorek, F. Ungar, A. M. Barth, A. Vagov, V. M. Axt. 'Path-integral approach for nonequilibrium multitime correlation functions of open quantum systems coupled to Markovian and non-Markovian environments'. *Phys. Rev. B* **98**, 125302 (2018). doi:10.1103/PhysRevB.98.125302.
[30] P. Machnikowski, V. M. Axt, T. Kuhn. 'Quantum-information encoding in dressed qubits'. *Phys. Rev. A* **75**, 052330 (2007). doi:10.1103/PhysRevA.75.052330.
[31] H. Carmichael. *An open systems approach to Quantum Opt.* Springer, Berlin (1993).
[32] A. Strathearn, P. Kirton, D. Kilda, J. Keeling, B. W. Lovett. 'Efficient non-Markovian quantum dynamics using time-evolving matrix product operators'. *Nat. Commun.* **9**, 3322 (2018). doi:10.1038/s41467-018-05617-3.
[33] C. Roy, S. Hughes. 'Influence of electron–acoustic-phonon scattering on intensity power broadening in a coherently driven quantum-dot–cavity system'. *Phys. Rev. X* **1**, 021009 (2011). doi:10.1103/PhysRevX.1.021009.
[34] A. Nazir, D. P. S. McCutcheon. 'Modelling exciton-phonon interactions in optically driven quantum dots'. *J. Phys.: Condens. Matter* **28**, 103002 (2016). doi:10.1088/0953-8984/28/10/103002.
[35] J. Iles-Smith, A. Nazir. 'Quantum correlations of light and matter through environmental transitions'. *Optica* **3**, 207 (2016). doi:10.1364/OPTICA.3.000207.
[36] K. Roy-Choudhury, S. Hughes. 'Quantum theory of the emission spectrum from quantum dots coupled to structured photonic reservoirs and acoustic phonons'. *Phys. Rev. B* **92**, 205406 (2015). doi:10.1103/PhysRevB.92.205406.
[37] C. Gustin, S. Hughes. 'Pulsed excitation dynamics in quantum-dot–cavity systems: Limits to optimizing the fidelity of on-demand single-photon sources'. *Phys. Rev. B* **98**, 045309 (2018). doi:10.1103/PhysRevB.98.045309.
